# Supplementary material for: Modeling the Influence of Solvation on the Electrochemical Double Layer of Salt / Solvent Mixtures
Source: arXiv:2408.04314 ancillary file (2024-08-08)
Supplement: Supplementary file 1 [file Solvation_on_EDL_SI.pdf]

# **Supporting Information:**

## **Modelling Solvation Structure in the Electrochemical Double Layer**

Constantin Schwetlick,<sup>†,‡</sup> Max Schammer,<sup>¶,†</sup> Arnulf Latz,<sup>¶,†,‡</sup> and Birger  
Horstmann<sup>\*,¶,†,‡</sup>

<sup>†</sup>*Helmholtz Institute Ulm, Helmholtzstraße 11, 89081 Ulm, Germany*

<sup>‡</sup>*Universität Ulm, Albert-Einstein-Allee 47, 89081 Ulm, Germany*

<sup>¶</sup>*German Aerospace Center, Wilhelm-Runge-Straße 10, 89081 Ulm, Germany*

E-mail: [birger.horstmann@dlr.de](mailto:birger.horstmann@dlr.de)

# Contents

|                                                                                                                                      |             |
|--------------------------------------------------------------------------------------------------------------------------------------|-------------|
| <b>S-1 Electrochemical Forces</b>                                                                                                    | <b>S-3</b>  |
| <b>S-2 Derivation of Independent Forces</b>                                                                                          | <b>S-4</b>  |
| <b>S-3 Removing dimensionality from the transport equations</b>                                                                      | <b>S-7</b>  |
| <b>S-4 Minimising the free energy with solvation</b>                                                                                 | <b>S-8</b>  |
| <b>S-5 Details on numerical implementation</b>                                                                                       | <b>S-10</b> |
| <b>S-6 Analytical Discussion of the Differential Capacitance</b>                                                                     | <b>S-12</b> |
| S-6.1 Symmetric Electrolytes Without Solvation: Influence of Dilution . . . . .                                                      | S-12        |
| S-6.2 Asymmetric Electrolytes Without Solvation: Influence of Solvent Size . . . . .                                                 | S-13        |
| S-6.3 Effective Dilution for Solvated Ions . . . . .                                                                                 | S-16        |
| <b>S-7 Differential Capacitance Without Solvation</b>                                                                                | <b>S-16</b> |
| <b>S-8 Nano-Structure of the EDL: Concentration Profiles</b>                                                                         | <b>S-17</b> |
| <b>S-9 Parameterisation for Validation</b>                                                                                           | <b>S-19</b> |
| <b>S-10 Influence of Dilution and Solvent Size on the Central Extremum of the Differential<br/>    Capacitance Without Solvation</b> | <b>S-20</b> |
| <b>References</b>                                                                                                                    | <b>S-22</b> |

## S-1 Electrochemical Forces

In this section, we present a brief derivation of the electrochemical forces based on our constitutive modelling. For a more detailed discussion, we refer to Refs. [S1–S3](#).

It has been shown in Ref. [S2](#) that the electrochemical forces  $\nabla\mu_\alpha^{\text{el}}$  follow from the free energy via constitutive equations  $\mu_\alpha = \partial(\rho\varphi_{\text{H}})/\partial c_\alpha$ , and by assuming incompressibility in the limiting case where inertial effects are neglected. Thus, our model free energy from above yields

$$\mu_{\alpha \neq \text{s}} = \nu_\alpha p^{\text{vol}} + RT \ln(c_\alpha/c^{\text{free}}) + RT\lambda_\alpha^{\text{m}} \left[ \tilde{E}_\alpha - \ln(x^{\text{free}} + \exp \tilde{E}_\alpha) \right] \quad (\text{S-1})$$

for the ions and

$$\mu_{\text{s}} = \nu_{\text{s}} p^{\text{vol}} + RT \ln x^{\text{free}} \quad (\text{S-2})$$

for the solvent species. Here,  $p^{\text{vol}} = \mathcal{K}(\sum_{\beta=1}^N \nu_\beta^0 c_\beta - 1)$  is the pressure resulting from excluded volume effects. The corresponding steric forces compete with electrostatic forces in charged regions of confined electrolytes, which determines the structure of the electrochemical double layer. [S3](#)

Apparently, the chemical potentials of the ion-species differ from the model without solvation by an additional contribution (last term in eq. (S-1)). [S2](#) In contrast, the chemical potential of all solvent species (bound, or free) equal the chemical potential of the unbound "free" solvent derived from a model without solvation (see eq. (S-2)).

Here, we focus on a kinematical description where the surface forces acting on the electrolyte system are in mechanical equilibrium. These surface forces are determined by the free energy density via a constitutive equation, [S2](#) and are comprised in the Cauchy stress tensor  $\boldsymbol{\sigma} = \boldsymbol{E} \otimes \boldsymbol{D} + \boldsymbol{\tau} - (p^{\text{elastic}} + \boldsymbol{E}\boldsymbol{D}/2) \cdot \mathbf{1}$ . The viscosity tensor  $\boldsymbol{\tau}$  accounts for irreversible momentum dissipation due to internal friction. In contrast, the elastic pressure  $p^{\text{elastic}} = \rho^2 \cdot \partial\varphi_{\text{H}}/\partial\rho = \sum_\alpha c_\alpha \mu_\alpha - \rho\varphi_{\text{H}}$  is a thermodynamic quantity, which comprises elastic deformations, and is determined by the free energy density. However, it follows from eqs. (S-1) and (6) that, although the mixing entropy

and the energy of solvation contribute to  $\rho\varphi_H$ , they do not contribute to  $p^{\text{elastic}}$ . Thus, solvation processes do not lead to pressure forces, and the stress tensor reduces to

$$\boldsymbol{\sigma} = \boldsymbol{\Sigma} + \boldsymbol{\tau} - p^{\text{vol}} \cdot \mathbf{1}, \quad (\text{S-3})$$

where  $\boldsymbol{\Sigma} = \mathbf{E} \otimes \mathbf{D} - (\mathbf{E}\mathbf{D}/2) \cdot \mathbf{1}$  is the Maxwell stress tensor. We assume that inertial effects  $\rho\dot{\mathbf{v}} = \nabla\boldsymbol{\sigma}$  can be neglected to a good approximation, such that  $\nabla p^{\text{vol}} = -\varrho\nabla\Phi + \nabla\boldsymbol{\tau}$ . Thus, the steric pressure forces are balanced by electrostatic forces and by viscous friction-forces. Furthermore, we assume that the partial molar volumes do not depend on pressure forces. This constitutes an incompressible limit for the hardly compressible liquid electrolytes,<sup>S2</sup> in which all forces are well-defined. Altogether, we find

$$\nabla\mu_\alpha^{\text{el}}|_{\alpha \neq s} = (Fz_\alpha - \nu_\alpha\varrho)\nabla\Phi + RT\left(\nabla\ln\left[c_\alpha/c^{\text{free}}\right] - \lambda_\alpha^{\text{m}}\nabla\ln\left[x^{\text{free}} + \exp(\tilde{E}_\alpha)\right]\right) + \nu_\alpha\nabla\boldsymbol{\tau}, \quad (\text{S-4})$$

and

$$\nabla\mu_s^{\text{el}} = (Fz_s - \nu_s\varrho)\nabla\Phi + RT\nabla\ln x^{\text{free}} + \nu_s\nabla\boldsymbol{\tau}. \quad (\text{S-5})$$

By construction, the forces  $\nabla\mu_\alpha$  satisfy the relation  $\sum_{\alpha=1}^N c_\alpha \nabla\mu_\alpha^{\text{el}} = \nabla\boldsymbol{\tau}$ . However, because the viscosity tensor  $\boldsymbol{\tau}$  is an isotropic function of the velocity gradient,<sup>S2</sup> we neglect the frictional contribution  $\nabla\boldsymbol{\tau}$  in our stationary description.

## S-2 Derivation of Independent Forces

In this section, we derive the set of independent thermodynamic forces appearing in our constitutive modelling. Our derivation is based on the continuum framework presented in great detail in Ref. S2 and Ref. S1.

Because we use an Onsager approach, the modelling of the thermodynamic fluxes and the

forces is coupled, as can be seen in the entropy production rate  $\mathcal{R}$  which contains the contribution

$$\mathcal{R}^{\text{flux}} = - \sum_{\alpha=1}^N \mathcal{N}_{\alpha}^{\text{CMF}} \cdot \nabla \mu_{\alpha}^{\text{el}}. \quad (\text{S-6})$$

The quantity  $\mathcal{R}$  plays a crucial role in our constitutive modeling. It couples the entropy principle imposed upon the entropy evolution by the second law of thermodynamics with fundamental balancing laws, e.g., for energy and momentum, via the condition that  $\mathcal{R} \geq 0$ .

The fluxes  $\mathcal{N}_{\alpha}^{\text{CMF}} = c_{\alpha}(\mathbf{v}_{\alpha} - \mathbf{v}^{\text{CMF}})$  appearing in eq. (S-6) are defined with respect to the center-of-mass convection velocity, defined by  $\rho \mathbf{v}^{\text{CMF}} = \sum_{\alpha=1}^N \rho_{\alpha} \mathbf{v}_{\alpha}$ , where  $\rho = \sum_{\beta=1}^N \rho_{\beta}$ . The center-of-mass frame (CMF) constitutes the specific frame of reference, which is related to the principle of momentum balance. However, as it was shown in Ref. S1, we can transform to alternative frames of reference. The choice of the reference frame can be motivated by the properties of the specific system under consideration. For incompressible systems, the frame of reference based on the volume averaged convection velocity  $\mathbf{v}^{\text{vol}} = \sum_{\alpha=1}^N c_{\alpha} \mathbf{v}_{\alpha}$  is very useful.<sup>S4,S5</sup> The corresponding volume flux is related to the CMF via

$$\mathcal{N}_{\alpha}^{\text{vol}} = \mathcal{N}_{\alpha}^{\text{CMF}} - c_{\alpha} (\mathbf{v}^{\text{vol}} - \mathbf{v}^{\text{CMF}}). \quad (\text{S-7})$$

In any frame of reference, there exists a flux constraint, which reduces the number of independent fluxes by one. The corresponding flux constraint in the volume averaged description reads  $\sum_{\alpha=1}^N \mathbf{v}_{\alpha} \cdot \mathcal{N}_{\alpha}^{\text{vol}} = 0$ . We use this condition and designate the flux related to the solvent species such that

$$\mathcal{N}_s^{\text{vol}} = - \sum_{\alpha \neq s}^N \mathbf{v}_{\alpha} \cdot \mathcal{N}_{\alpha}^{\text{vol}}. \quad (\text{S-8})$$

By construction, the transformation between the CMF and the volume averaged frame can be expressed via  $\mathbf{v}^{\text{vol}} - \mathbf{v}^{\text{CMF}} = - \sum_{\alpha=1}^N \mathcal{N}_{\alpha}^{\text{vol}} \cdot M_{\alpha} / \rho$ , where  $M_{\alpha}$  is the specific molar mass. Using eq. (S-8), we thus find

$$\mathbf{v}^{\text{vol}} - \mathbf{v}^{\text{CMF}} = - \frac{1}{\rho} \sum_{\alpha \neq s} \mathcal{N}_{\alpha}^{\text{vol}} \left( M_{\alpha} - M_s \cdot \frac{\mathbf{v}_{\alpha}}{\mathbf{v}_s} \right) \quad (\text{S-9})$$

In our approach, we obtain the thermodynamic forces from the model of the free energy density  $\rho\phi_H$  and via neglecting inertial contributions in the force-law (see Ref. S2). Based on the solvation model for the free energy density presented in the main text (see eq. (6)), we find

$$\nabla\mu_\alpha^{\text{el}}|_{\alpha \neq s} = (Fz_\alpha - \nu_\alpha \varrho) \nabla\Phi + RT \left( \nabla \ln \left[ c_\alpha / c^{\text{free}} \right] - \lambda_\alpha^{\text{m}} \nabla \ln \left[ x^{\text{free}} + \exp(\tilde{E}_\alpha) \right] \right) + \nabla\mathbf{t}, \quad (\text{S-10})$$

and

$$\nabla\mu_s^{\text{el}} = (Fz_s - \nu_s \varrho) \nabla\Phi + RT \nabla \ln x^{\text{free}} + \nabla\mathbf{t}. \quad (\text{S-11})$$

However, these quantities are mutually coupled via the condition  $\sum_{\alpha=1}^N c_\alpha \cdot \nabla\mu_\alpha^{\text{el}} = \nabla\mathbf{t}$ . We make use of this constraint and solve for the solvent species,

$$c_s \cdot \nabla\mu_s^{\text{el}} = \nabla\mathbf{t} - \sum_{\alpha \neq s}^N c_\alpha \cdot \nabla\mu_\alpha^{\text{el}}. \quad (\text{S-12})$$

We make use of eqs. (S-8), (S-9) and (S-12) and express the right side of eq. (S-6) via the volume-averaged description via substitution,

$$\mathcal{R}^{\text{flux}} = - \sum_{\alpha \neq s}^N \mathcal{N}_\alpha^{\text{vol}} \cdot \xi_\alpha, \quad (\text{S-13})$$

where the N-1 independent forces are determined by the constitutive equation

$$\xi_\alpha = \left( z_\alpha - z_s \frac{\nu_\alpha}{\nu_s} \right) F \nabla\Phi + \sum_{\beta \neq s} \left( \delta_\beta^\alpha + \frac{c_\beta}{c_s} \frac{\nu_\alpha}{\nu_s} \right) \cdot \nabla \left( \frac{\partial}{\partial c_\beta} \left[ \rho\phi_H^{\text{mixing}} + \rho\phi_H^{\text{solvation}} \right] \right) + \left( M_\alpha - M_s \frac{\nu_\alpha}{\nu_s} \right) \frac{\nabla\mathbf{t}}{\rho}, \quad (\text{S-14})$$

where  $\rho\phi_H^{\text{mixing}}$  and  $\rho\phi_H^{\text{solvation}}$  are contributions to the free energy density stemming from the entropy of mixing and the solvation binding energy, see Ref. S2. Equation (S-13) gives rise to an Onsager approach, where the fluxes  $\mathcal{N}_\alpha^{\text{vol}}$  are expressed as linear functions of the independent forces  $\xi_\alpha$ .

We stated our model for the mixing entropy and the solvation binding energy in the main text, see eq. (6). Furthermore, for the description of the equilibrium structures of the EDL, we neglect the viscous term appearing on the right side of eq. (S-14). Using  $c_s^{\text{bound}} = \sum_{\alpha=\pm} \lambda_{\alpha}^m c_{\alpha} \cdot x^{\text{free}} / (x^{\text{free}} + \exp \tilde{E}_{\alpha})$  and  $c^{\text{free}}(1 - x^{\text{free}}) = c_+ + c_-$ , we find for the corresponding forces

$$\xi_{\alpha \neq s} = \left( z_{\alpha} - \frac{\nu_{\alpha}}{\nu_s} z_s \right) F \nabla \Phi + RT \nabla \left( \ln(1 - x^{\text{free}}) - \frac{\nu_{\alpha}}{\nu_s} \ln(x^{\text{free}}) - \lambda_{\alpha}^m \ln(x^{\text{free}} + \exp[\tilde{E}_{\alpha}]) + \ln \left[ \frac{c_{\alpha}}{\sum_{\beta \neq s} c_{\beta}} \right] \right). \quad (\text{S-15})$$

Next, we focus on equilibrium structures of the electrochemical double layer (EDL). For this purpose, it suffices to discuss the stationary state, in which all fluxes become constant.<sup>S3</sup> Hence, the fluxes are completely determined by the boundary conditions.<sup>S3,S6</sup> We make use of this property, and assume vanishing fluxes at the electrode, which implies that the fluxes vanish everywhere.<sup>S2</sup> Because we use an Onsager approach in our framework, where the fluxes are linear functions of the electrochemical forces,<sup>S2</sup> if the independent forces vanish, this is sufficient to ensure a stationary state with no fluxes  $\mathcal{N}_{\alpha}$  and  $\mathcal{J} = \sum_{\alpha} z_{\alpha} \mathcal{N}_{\alpha}$ .<sup>S3</sup> The electrochemical forces follow directly from the model free energy (see section S-1). However, for the EDL description of an electrolyte with N species, only N-1 forces  $\xi_{\alpha}$  are independent (see section S-2). By convention, we omit the force related to the solvent, such that the resulting set of N stationary EDL equations (for an electrolyte mixture composed on N species) consists of N-1 trivial force equations, supplemented by Poisson's equation

$$\xi_{\alpha \neq s} = 0, \quad \text{and} \quad \varrho = -\varepsilon_0 \nabla (\varepsilon_R \nabla \Phi). \quad (\text{S-16})$$

We state the constitutive equation for the forces in section S-2.

### S-3 Removing dimensionality from the transport equations

We consider here a three species electrolyte consisting of a neutral solvent and a dissociated salt, i.e. a cation and an anion species, as described in section II B. The stationary solution with no fluxes across the electrode surface can be described by three equations, two force equations  $\xi_{\alpha} = 0$

and the Poisson equation.

In order to simplify our description, we remove the physical dimensions from the variables. From now on,  $\tilde{\Phi} = Fz_+ \Phi / RT$ ,  $\tilde{\varrho} = \nu_{\text{salt}} \varrho / Fz_+$ ,  $\tilde{c}_s = c_s \nu_{\text{salt}}$ , and  $\tilde{c}_{\pm}(\tilde{\varrho}, \tilde{c}_s) = c_{\pm} \nu_{\text{salt}}$  are dimensionless variables. Expressed via the independent quantities  $\tilde{\varrho}$  and  $\tilde{c}_s$ , we find for the ion concentrations

$$\tilde{c}_{\pm} = 1 \pm \gamma_{\mp} \tilde{\varrho} - \tilde{c}_s. \quad (\text{S-17})$$

According to this convention, we get an expression for the Debye-length,<sup>S3</sup>  $L_D = \sqrt{RT \epsilon_0 \epsilon_R \nu_{\text{salt}} / (Fz_+)^2}$ .

Via this length scale, we remove the physical dimensions from the differential operator,  $\tilde{\nabla} = L_D \nabla$ , such that Poisson's equation reads  $\tilde{\varrho} = -\tilde{\nabla}^2 \tilde{\Phi}$ . Furthermore, the non-dimensional forces  $\tilde{\xi}_{\alpha} = L_D \xi_{\alpha} / RT$  read

$$\tilde{\xi}_{\pm} = \pm \tilde{\nabla} \tilde{\Phi} + \tilde{\nabla} \left( \ln(1-x) - \lambda_{\pm}^m \ln(x + \exp \tilde{E}_{\pm}) - \frac{\gamma_{\pm}}{\gamma_s} \ln x + \ln \frac{\tilde{c}_{\pm}}{\tilde{c}_{\text{IL}}} \right) \quad (\text{S-18})$$

where  $\tilde{c}_{\text{IL}} = \tilde{c}_+ + \tilde{c}_-$ . In principle, in the stationary state where  $\tilde{\xi}_{\pm} = 0$  (see section III), the two forces in eq. (S-18) can be integrated using electroneutral boundary conditions for the bulk. This then yields two algebraic expressions, which are supplemented by the Poisson equation.

## S-4 Minimising the free energy with solvation

The free energy including solvation has the form

$$\begin{aligned} \rho \varphi_H = RT \sum_{\alpha \neq s}^N c_{\alpha} \lambda_{\alpha}^m & \left( \tilde{\lambda}_{\alpha} \ln(\tilde{\lambda}_{\alpha}) + (1 - \tilde{\lambda}_{\alpha}) \ln(1 - \tilde{\lambda}_{\alpha}) + \tilde{\lambda}_{\alpha} \tilde{E}_{\alpha} \right) \\ & + RT \left( \sum_{\alpha \neq s}^N c_{\alpha} \ln \frac{c_{\alpha}}{c^{\text{free}}} + c_s^{\text{free}} \ln \frac{c_s^{\text{free}}}{c^{\text{free}}} \right) \\ & + \frac{\mathcal{K}}{2} \left( 1 - \sum_{\alpha=1}^N c_{\alpha} \nu_{\alpha}^0 \right)^2 + \frac{\mathbf{E} \mathbf{D}}{2}. \quad (\text{S-19}) \end{aligned}$$

$c_s^{\text{free}}$  is given by  $c_s - \sum_{\alpha} c_{\alpha} \lambda_{\alpha}^m \tilde{\lambda}_{\alpha}$ , the solvent concentration reduced by the concentration of bound solvent. Similarly  $c^{\text{free}} = c_s + \sum_{\alpha} c_{\alpha} (1 - \lambda_{\alpha}^m \tilde{\lambda}_{\alpha})$ . This contains the variables  $\tilde{\lambda}$ , for which we have

to solve first. To do so, we assume that the equilibrium between bound solvent and free solvent is established at a much shorter timescale than that of diffusion. Note that this short timescale equilibrium only takes into account whether the solvent is bound in the inner solvation shell of an ion, therefore to change its status from bound to free the solvent only has to move on the order of Å.

The equilibrium is assumed to be established to minimise the free energy with respect to the solvation contribution. All parts which depend on the coordination numbers can be collected in

$$\begin{aligned}\mathcal{L} = & c_s^{\text{free}} \ln c_s^{\text{free}} - c^{\text{free}} \ln c^{\text{free}} + \lambda_+^m \tilde{\lambda}_+ c_+ \ln \tilde{\lambda}_+ + (1 - \tilde{\lambda}_+) \lambda_+^m c_+ \ln(1 - \tilde{\lambda}_+) \\ & + \lambda_-^m \tilde{\lambda}_- c_- \ln \tilde{\lambda}_- + (1 - \tilde{\lambda}_-) \lambda_-^m c_- \ln(1 - \tilde{\lambda}_-) + \lambda_+^m \tilde{\lambda}_+ c_+ \tilde{E}_+ + \lambda_-^m \tilde{\lambda}_- c_- \tilde{E}_-\end{aligned}\quad (\text{S-20})$$

The minimum in the free energy can be found by taking the derivatives with respect to the variables we want to solve for:

$$\frac{\partial \mathcal{L}}{\partial \tilde{\lambda}_+} = \lambda_+^m c_+ \left( -\ln c_s^{\text{free}} - 1 + \ln c^{\text{free}} + 1 + \ln \tilde{\lambda}_+ + 1 - \ln(1 - \tilde{\lambda}_+) - 1 + \tilde{E}_+ \right) \quad (\text{S-21})$$

$$\frac{\partial \mathcal{L}}{\partial \tilde{\lambda}_-} = \lambda_-^m c_- \left( -\ln c_s^{\text{free}} - 1 + \ln c^{\text{free}} + 1 + \ln \tilde{\lambda}_- + 1 - \ln(1 - \tilde{\lambda}_-) - 1 + \tilde{E}_- \right) \quad (\text{S-22})$$

As both  $c_{\pm}$  are always positive, the terms in the brackets have to equal 0. Defining a solvation parameter  $x^{\text{free}} \equiv \frac{c_s^{\text{free}}}{c^{\text{free}}}$ , which describes the fraction of free solvent in all free particles, we see

$$\frac{\tilde{\lambda}_+}{1 - \tilde{\lambda}_+} e^{\tilde{E}_+} = \frac{\tilde{\lambda}_-}{1 - \tilde{\lambda}_-} e^{\tilde{E}_-} = x^{\text{free}}, \quad \text{so} \quad (\text{S-23})$$

$$\tilde{\lambda}_\alpha = \frac{x^{\text{free}}}{x^{\text{free}} + \exp(\tilde{E}_\alpha)} \quad (\text{S-24})$$

This determines  $\tilde{\lambda}_{\pm}$  as a function of  $x^{\text{free}}$ . Combining,  $x^{\text{free}}$  is then given by the solution to the equation  $x^{\text{free}} = \frac{c_s^{\text{free}}}{c^{\text{free}}}$ , in general a third order polynomial for three species.

## S-5 Details on numerical implementation

The results presented in the paper were obtained from a numerical implementation of our model in a static configuration, as described in section III.

The equations to be solved were a set of 4 linear differential equations in the case of a 3 species electrolyte. They can be written down in a matrix notation of the form

$$\begin{pmatrix} \xi_+ \\ \xi_- \\ E \\ \frac{\varrho}{F} \end{pmatrix} = A(\varrho, c_s) \cdot \begin{pmatrix} \nabla \Phi \\ \nabla \frac{\varrho}{F} \\ \nabla c_+ \\ \nabla E \end{pmatrix}. \quad (\text{S-25})$$

The matrix  $A$  including solvation is known as a function of the gradients  $(\nabla \Phi, \nabla x^{\text{free}}, \nabla c_+, \nabla c_-, \nabla E)$ :

$$A^R = \begin{pmatrix} z_+ F & -RT \left( \frac{1}{1-x^{\text{free}}} + \frac{\lambda_+^m}{x^{\text{free}} + \exp \bar{E}_+} + \frac{\nu_+}{\nu_s x^{\text{free}}} \right) & RT \left( \frac{1}{c_+} - \frac{1}{c_+ + c_-} \right) & -RT \frac{1}{c_+ + c_-} & 0 \\ z_- F & -RT \left( \frac{1}{1-x^{\text{free}}} + \frac{\lambda_-^m}{x^{\text{free}} + \exp \bar{E}_-} + \frac{\nu_-}{\nu_s x^{\text{free}}} \right) & -RT \frac{1}{c_+ + c_-} & RT \left( \frac{1}{c_-} - \frac{1}{c_+ + c_-} \right) & 0 \\ -1 & 0 & 0 & 0 & 0 \\ 0 & 0 & 0 & 0 & \frac{\varepsilon_0 \varepsilon_R}{F} \end{pmatrix} \quad (\text{S-26})$$

To transform this matrix into the required base of  $(\nabla \Phi, \nabla \varrho/F, \nabla c_+, \nabla E)$  we use another set of matrices to switch bases. First, the solvation parameter  $x^{\text{free}}$  is replaced by the species concentrations in  $R^{x^{\text{free}}}$ , which is given with respect to  $(\nabla \Phi, \nabla c_s, \nabla c_+, \nabla c_-, \nabla E)$ :

$$R^{x^{\text{free}}} = \begin{pmatrix} 1 & 0 & 0 & 0 & 0 \\ 0 & \frac{\partial x^{\text{free}}}{\partial c_s} & \frac{\partial x^{\text{free}}}{\partial c_+} & \frac{\partial x^{\text{free}}}{\partial c_-} & 0 \\ 0 & 0 & 1 & 0 & 0 \\ 0 & 0 & 0 & 1 & 0 \\ 0 & 0 & 0 & 0 & 1 \end{pmatrix}, \quad (\text{S-27})$$

where

$$\frac{\partial x^{\text{free}}}{\partial c_s} = \frac{1 - x^{\text{free}}}{C_x}, \text{ and } \frac{\partial x^{\text{free}}}{\partial c_{\pm}} = \frac{-x^{\text{free}} - (1 - x^{\text{free}})\lambda_{\pm}}{C_x}, \quad (\text{S-28})$$

with

$$C_x = c_s + c_+ + c_- - \lambda_+ c_+ - \lambda_- c_- + \frac{(1 - x^{\text{free}})(\lambda_+^{\text{m}} - \lambda_+)}{x^{\text{free}} + \exp \tilde{E}_+} c_+ + \frac{(1 - x^{\text{free}})(\lambda_-^{\text{m}} - \lambda_-)}{x^{\text{free}} + \exp \tilde{E}_-} c_- \quad (\text{S-29})$$

This is dependent on the local variables, so has to be recalculated for every numerical step. The transformation to the final base  $(\nabla\Phi, \nabla\frac{\varrho}{F}, \nabla c_+, \nabla E)$  is done with a second matrix

$$R^{\varrho} = \begin{pmatrix} 1 & 0 & 0 & 0 \\ 0 & -\frac{\nu_-}{\tilde{\nu}_s z_-} & \frac{\nu_- z_+ - \nu_+ z_-}{\tilde{\nu}_s z_-} & 0 \\ 0 & 0 & 1 & 0 \\ 0 & \frac{\nu_s}{\tilde{\nu}_s z_-} & \frac{\nu_+ z_s - \nu_s z_+}{\tilde{\nu}_s z_-} & 0 \\ 0 & 0 & 0 & 1 \end{pmatrix}. \quad (\text{S-30})$$

Here  $\tilde{\nu}_s = \nu_s - \nu_- \frac{z_s}{z_-}$ , a molar volume reflecting charge conservation constraints. [S2](#)

$A$  can therefore be expressed as

$$A = A^R R^{x^{\text{free}}} R^{\varrho}. \quad (\text{S-31})$$

As the left hand side of eq. (S-25) is based on known values (the forces are set to 0,  $E$  and  $\varrho$  can be calculated from the previous step), the gradients on the right hand side can be calculated by inverting  $A$ .

The code to solve these equations was written in MATLAB using the ode15s solver for stiff differential equations. The tolerances were set at  $1 \times 10^{-8} \text{ V m}^{-1}$  for  $E$ ,  $1 \times 10^{-14} \text{ V}$  for  $\Phi$  and  $1 \times 10^{-13} \text{ mol/m}^3$  for both  $\varrho/F$  and  $c_+$ . The solver chooses variable step sizes to maintain these tolerances. As mentioned in section III, the bulk vector has to be chosen to be nonzero to avoid the trivial solution. For this reason,  $E^{\text{b}} = \pm 0.1 \text{ V m}^{-1}$  was set while keeping  $\varrho^{\text{b}}$  at 0. The calculation

was stopped once propagating 500 nm from the bulk condition, and subsequently cut to the desired potential difference from electrode to bulk.

## S-6 Analytical Discussion of the Differential Capacitance

### S-6.1 Symmetric Electrolytes Without Solvation: Influence of Dilution

In this section, we focus on the influence of dilution on the differential capacitance (DC) in the EDL for the specific case of a symmetric electrolyte, where all species have the same volume. Via this analysis, we obtain analytical expressions for the charge density (i.e., ion concentrations) and the electric field inside the electrolyte as function of the electric potential. We show that our results reproduce the description proposed by [Kornyshev](#) in Ref. [S7](#). In this seminal publication, the author derived analytically the prediction that the critical value at which the DC profile transitions from a camel shape to a bell shape is  $\varphi^{\text{crit}} = 1/3$ . As mentioned in the main text, this matches exactly the results from our numerical simulations.

Assuming  $\gamma_{\pm} = \gamma_s = 0.5$  and neglecting solvation effects ( $\lambda_{\pm}^{\text{m}} = 0$ ) in the non-dimensional expression for the fluxes (see eq. (S-18)), we obtain for the two trivial forces

$$0 = \nabla \left( \pm \tilde{\Phi} + \log [\tilde{c}_{\pm}/\tilde{c}_s] \right). \quad (\text{S-32})$$

This can be integrated from the bulk region of the electrolyte towards the charged interface. Using electroneutral boundary conditions (see section III), we find  $\tilde{c}_{\pm} = \tilde{c}_s \cdot \exp(\mp \tilde{\Phi}) \cdot \varphi/(1 - \varphi)$ . Using  $\tilde{c}_{\pm} = 1 \mp \tilde{\varrho}/2 - \tilde{c}_s$  (see section II B),

$$\tilde{c}_{\pm} = \frac{1 \pm \tilde{\varrho}/2}{1 + (1 - \varphi) \exp(\pm \tilde{\Phi})/\varphi}. \quad (\text{S-33})$$

Hence, the two ion concentrations are related via  $\tilde{c}_{+} = \tilde{c}_{-} \cdot \exp(-2\tilde{\Phi})$ . By solving this for  $\tilde{\varrho} = \tilde{c}_{+} - \tilde{c}_{-}$  and using the relation  $\cosh \tilde{\Phi} = 1 + 2 \sinh^2(\tilde{\Phi}/2)$ , we obtain an analytical result for the charge

density as function of the electric potential,

$$\tilde{\rho}(\tilde{\Phi}) = -\frac{2\varphi \sinh \tilde{\Phi}}{1 + 2\varphi \sinh^2(\tilde{\Phi}/2)}. \quad (\text{S-34})$$

Alternatively, we can express eq. (S-34) via the dimensional ion concentrations, such that  $(c_+ - c_-) = -2c_{\text{salt}}^{\text{bulk}} \sinh(\tilde{\Phi})/(1 + 2\varphi \sinh^2[\tilde{\Phi}/2])$ . This is exactly the result presented by Kornyshev (see eq. (8) in S7). For electrolytes with non-vanishing amount of salt ( $\varphi > 0$ ), eq. (S-34) describes the profile of Fermi-Poisson equations. This becomes obvious, when we consider the profile of the ion concentrations

$$c_{\pm} = \frac{1}{2\nu_{\text{salt}}} \frac{\varphi \cdot \exp(\mp \tilde{\Phi})}{1 - \varphi + \varphi \cosh(\tilde{\Phi})}. \quad (\text{S-35})$$

Apparently, the ion concentrations cannot exceed their maximal "saturation" thresholds regardless of how large the polarization becomes,  $c_+(\tilde{\Phi} \rightarrow -\infty) = c_-(\tilde{\Phi} \rightarrow \infty) = c_{\pm}^{\text{sat}} = 1/\nu_{\text{salt}}$ .

The analytical result in eq. (S-34) can be used to derive an expression for the EDL charge  $\tilde{Q}(\tilde{V}^{\text{ext}})$  and the differential capacitance. This is a consequence of the additional coupling between the charge density and the electric potential comprised in the Poisson equation  $\tilde{\rho} = -\tilde{\Phi}''$ . Hence, in one dimension, this can be solved for  $[\tilde{E}(\tilde{\Phi})]^2 = -2 \int_{\tilde{\Phi}^{\text{bulk}}}^{\tilde{\Phi}(\tilde{x})} d\tilde{\Phi} \tilde{\rho}(\tilde{\Phi})$ , where the electric field is  $\tilde{E} = -\tilde{\Phi}'$ . Upon integration, this yields an expression for the EDL charge  $\tilde{Q}^{\text{EDL}} = \tilde{E}(\tilde{V}^{\text{ext}})$  and the differential capacitance  $\tilde{C}_{\delta} = d\tilde{Q}^{\text{EDL}}/d\tilde{V}^{\text{ext}}$  (here,  $\tilde{V}^{\text{ext}} = FV^{\text{ext}}/RT$ ). As shown in great detail in Ref. S7, this allows to derive the analytical result that the profile of  $\tilde{C}_{\delta}$  transitions from a camel shape (two peaks) to a bell shape (one peak) exactly if  $\varphi^{\text{crit}} = 1/3$ .

## S-6.2 Asymmetric Electrolytes Without Solvation: Influence of Solvent Size

In this section, we focus on the critical dilution for asymmetric electrolytes where the ions and solvent molecules do not have the same size.

In section S-6.1 we derived an analytical prediction for the critical dilution at which the profile of the differential capacitance transitions from a camel shape (two peaks) to a bell shape (one peak). However, the discussion presented there relied critically on the assumption that for all electrolyte

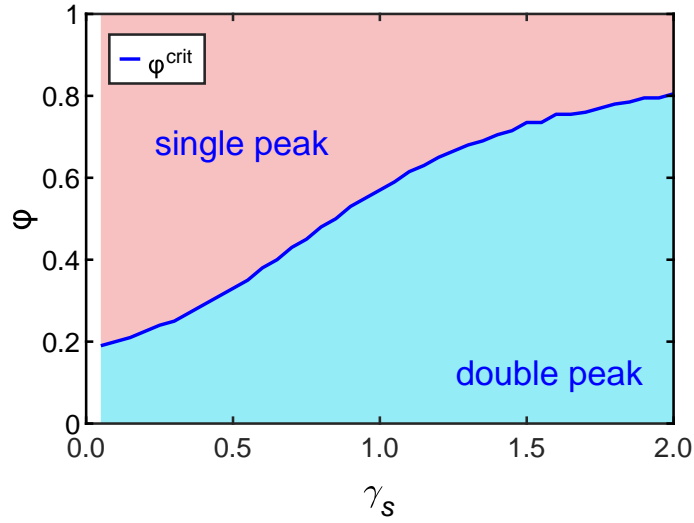

Figure S1: Phase diagram showing the critical dilution (i.e. transition from single peak to double peak in differential capacitance) for a symmetric salt ( $\gamma_{\pm} = 0.5$ ).

species  $\gamma_{\alpha} = 0.5$ . The analytical prediction for  $\phi^{crit}$  reproduced results from the literature, and was in accordance with our numerical results (see section IV B). However, for all electrolytes where the ions and the solvent molecules do not have the same size, the critical dilution will have another value which depends upon the size of the ions and the solvent molecules (see section IV B). In particular, the analytical discussion presented in section S-6.1 becomes more complex in the asymmetric case. For this reason, we instead focus on the results for the critical dilution obtained from numerical simulations.

To numerically obtain  $\phi^{crit}$ , EDL simulations have to be run for a large array of electrolyte parameters (here we varied  $\gamma_s$  between 0.05 and 2 in steps of 0.05 and  $\phi$  between 0.01 and 0.85 in steps of 0.01). By counting the maxima the resulting differential capacitance plots present, the phase boundary, at which the "camel"- "bell"-transition occurs, can be determined.

Figure S1 shows the critical dilution (blue curve) for an electrolyte with symmetric ions ( $\gamma_{\pm} = 0.5$ ), as function of the parameter space spanned by the dilution and relative size of the solvent molecules  $\gamma_s = v_s/v_{salt}$ . Here, the curve for  $\phi^{crit}$  indicates the transition from camel shape to bell shape; the region below the curve corresponds to the solvent sizes at which the DC profile has camel shape, whereas the region above the curve corresponds to the solvent sizes at which the DC

profile has camel shape. Apparently, the DC exhibits a camel shaped profile for high salt amounts only if the solvent molecules are larger than the ions. In contrast, for smaller solvent molecules, the DC profile is camel shaped only for highly diluted electrolytes (small  $\varphi$ ). The completely symmetric case, for which we derived analytical solution in section S-6.1), is given at  $\gamma_s = 0.5$  where the critical dilution is  $\varphi^{\text{crit}} = 1/3$ . Increasing the solvent size also increases the size of the double peak region. The largest solvent shown, which has twice the molar volume of the salt (i.e. 4 times as large as the ions) exhibits the "camel"-shape up to a dilution of  $\varphi = 0.8$ .

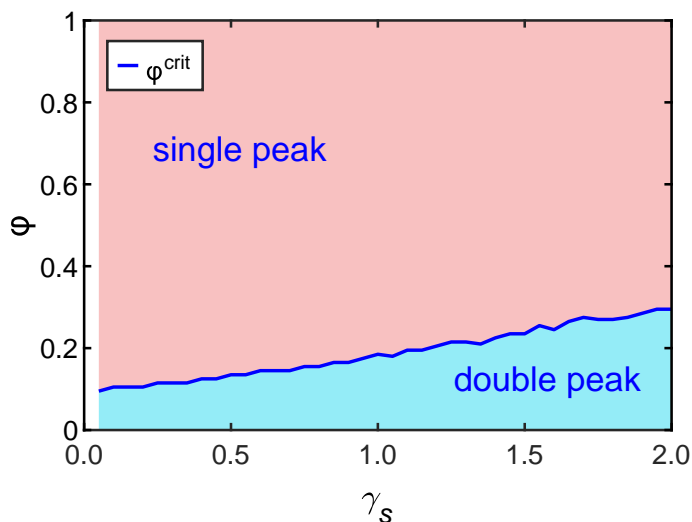

Figure S2: Phase diagram showing the critical dilution for an asymmetric salt ( $\gamma_+ = 0.9, \gamma_- = 0.1$ ).

Figure S2 shows a similar phase diagram, but for an asymmetric salt, in which the cations are significantly larger than the anions ( $\gamma_+ = 0.9$ ). Across all solvent sizes, the critical dilution is now lower. This is due to the asymmetric peak heights (see fig. 4), which means the minimum merges much earlier with the smaller peak. Nonetheless, the transition occurs at higher salt concentrations for larger solvents here as well.

Altogether, we thus conclude that, regardless of the relative ion sizes, larger solvents stabilise the "camel"-phase, where the differential capacitance has two maxima slightly displaced from the pzc.

### S-6.3 Effective Dilution for Solvated Ions

In this section, we pick up our discussion presented in section IV C. There, we rationalised our observation that the critical dilution decreases in the case of solvation by accounting for the size of the solvation shell via  $\varphi^{\text{eff}} = c_{\text{salt}}^{\text{bulk}} (\nu_{\text{salt}} + \lambda_{\text{salt}}^{\text{bulk}} \nu_s)$ .

In the case of infinite dilution and strong ion-solvent binding forces, the coordination number becomes equal to the maximum coordination number set in the model parameters  $\lambda_{\alpha}^{\text{m}}$ . This becomes clear when considering the equation for the coordination number  $\tilde{\lambda}_{\alpha} = \frac{x^{\text{free}}}{x^{\text{free}} + \exp \tilde{E}_{\alpha}}$ , as now  $x^{\text{free}} = c_s^{\text{free}} / c^{\text{free}} \gg 0$ . Requiring strong binding energy makes  $\exp \tilde{E}_{\alpha}$  vanish with respect to  $x^{\text{free}}$ , so  $\tilde{\lambda}_{\alpha} \rightarrow 1$ . Let us consider the electrolyte shown in fig. 5, with  $\lambda_{\pm}^{\text{m}} = 4$  and  $\gamma_s = \gamma_{\pm} = 0.5$ . Accounting for the size of the solvation shell, the effective dilution in the dilute limit is  $\varphi^{\text{eff}} = (\lambda_{\pm}^{\text{m}} + 1)\varphi = 5\varphi$ . However, the relative size of the solvent to the salt changes as well, so  $\gamma_s^{\text{eff}} = \gamma_s/5$ . In fig. 5 we see, that for this electrolyte the 'camel'-'bell'-transition occurs at a critical dilution  $\varphi_{\text{crit}} = 0.04$ . This corresponds to an effective dilution of  $\varphi_{\text{crit}}^{\text{eff}} = 0.2$ . Comparing this with the plot shown in fig. S1, at the effective relative solvent size of  $\gamma_s^{\text{eff}} = 0.1$ , we indeed see a critical dilution value of  $\varphi_{\text{crit}} = 0.2$ .

## S-7 Differential Capacitance Without Solvation

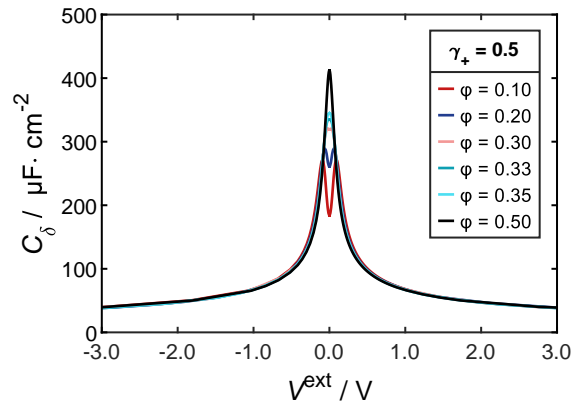

Figure S3: Differential capacitance plot of a symmetric salt ( $\gamma_+ = \gamma_- = \gamma_s = 0.5$ ) without solvation effects.

In the main text, we argued that the peaks of the DC profile appearing at higher potentials in

the case of solvation (see fig. 5) are due to the stripping of the solvation shell. Our reasoning was based on the argument that no such peaks are visible in the DC profile for the case without solvation. However, the specific figure appearing in the main text, see fig. 3, shows a rather small potential window. For consistency, we thus present here the same results, but for a larger potential window in fig. S3. Apparently, no additional peaks occur at larger potentials without solvation.

## S-8 Nano-Structure of the EDL: Concentration Profiles

Section IV C describes the structure of the EDL when solvation effects are taken into account. There we detail, how the salt concentration has a significant influence on the desolvation potential, at which the ions are stripped of their solvation shells. We argue, that this change in EDL structure from dilute to concentrated electrolytes arises from the lack of free solvent in concentrated electrolytes. In this section we present various concentration plots to reinforce our previous observations with a wider variety of electrolyte systems. All plots show the structure created by an external potential difference of 1 V between electrode and bulk electrolyte and assume an inert electrode.

Figure S4a depicts a rather dilute electrolyte with  $\varphi = 0.15$ , so the salt takes up 15% of the volume in the bulk. In this case the maximum of the bound solvent concentration in the intermediate region is still clearly visible. Further away from the electrode, the Stern layer follows, where both ions display exponential concentration profiles, while the solvent concentration remains constant. Closest to the electrode surface is a region, where only the anion (i.e. the screening counter-ion) is present in saturation. This can be considered a Helmholtz layer.

In fig. S4b a slightly more concentrated electrolyte ( $\varphi = 0.2$ ) can be seen. The intermediate region has become less pronounced, but all three are still present. The free solvent has now become scarce, reducing the increase in bound solvent in the intermediate region.

Figure S4c shows an electrolyte with dilution  $\varphi = 0.3$ . Here the intermediate region has all but disappeared, only noticeable in the slight change of the concentration gradient. The maximum in

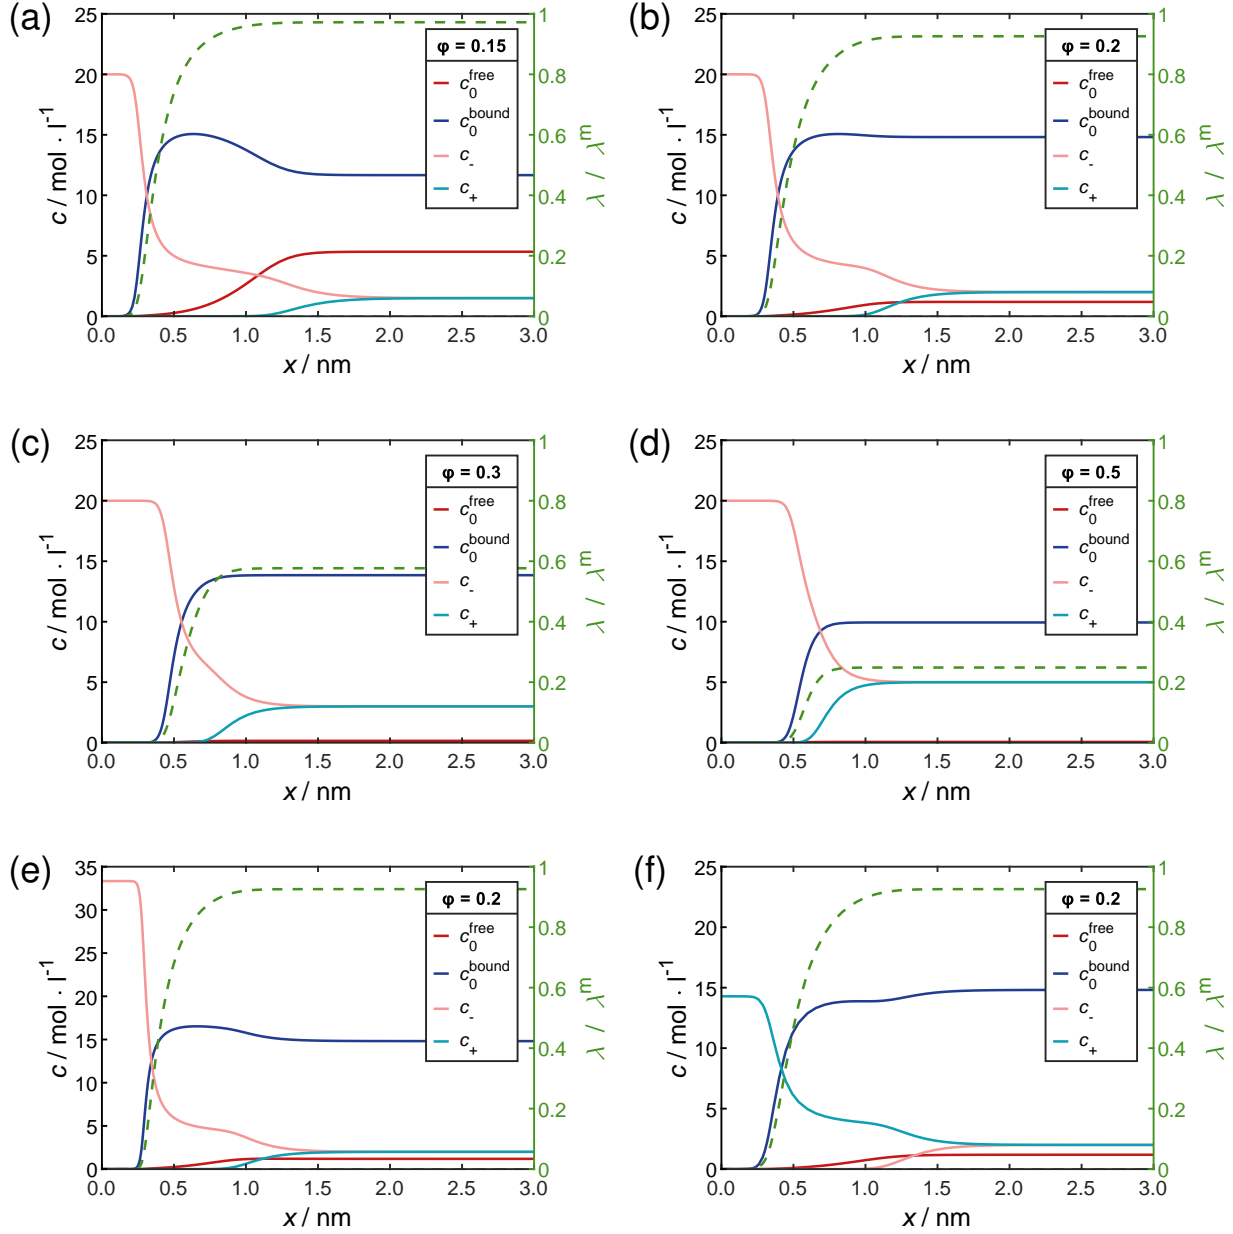

Figure S4: Concentration profiles in the EDL. Figure S4a to S4d show results for symmetric electrolytes at different dilutions  $\phi$  at  $V^{\text{ext}} = 1 \text{ V}$ , while fig. S4e and S4f depict an asymmetric electrolyte ( $\gamma_+ = 0.7$ ) for both a positively and negatively charged interface ( $V^{\text{ext}} = \pm 1 \text{ V}$ ).

the bound solvent concentration, however, has vanished. The Stern layer with the constant solvent concentration is still visible though. The disappearance of the intermediate layer coincides with there not being enough solvent to completely fill the solvation shells of the ions. As a consequence, the free solvent concentration is reduced to close to 0.

Finally, fig. S4d shows an extremely concentrated electrolyte, where the salt takes up half the total volume in the bulk. Noticeably, there is only enough solvent to fill the solvation shells to less than a third and no intermediate region.

As we increase the salt concentration the double layer can be seen to get thinner, and switched from a three layer profile to only two layers for very concentrated electrolytes. The order in which the species are removed from the EDL, however, remains the same: First the ion of equal charge to the electrode is forced out, then the free solvent, finally followed by the solvent bound to the counter-ion in solvation shells.

The two final figures fig. S4e and fig. S4f illustrate how ion size asymmetry influences the EDL-profile. In fig. S4e a positive charge is applied to the interface, therefore the anion is attracted to the electrode. This is assumed to be smaller than the cation, so it saturates at a higher concentration. The larger cation and the resulting smaller charge density in fig. S4f also increases the EDL-thickness. Depending on the ion size, the intermediate region plateau of the concentration of the bound solvent can either be higher or lower than the bulk value. But irrespective of ion asymmetry, the species still leave the EDL in the same order as described above.

## S-9 Parameterisation for Validation

In this section, we provide supplementary information regarding the parameterisation of the numerical simulations performed in section V C.

For the validation we used data obtained from Ref. S8 for the dielectric constant  $\epsilon = 46.7$ , and the molar volume of the solvent  $v_s = 7.1 \times 10^{-5} \text{ m}^3/\text{mol}$ . However, in order to account for steric effects in the solvation shell, we use a molar volume twice as large for our simulation. To estimate the size of the salt, the ionic radius quoted by Pal in Ref, S9 as  $5.44 \text{ \AA}$  for  $\text{PF}_6$  in an ionic liquid was converted to a molecular volume of  $4.1 \times 10^{-4} \text{ m}^3/\text{mol}$ . Assuming a potassium ion of equal size and a maximum solvent coordination number of 4 for  $\text{K}^+$  and 0 for  $\text{PF}_6$  (i.e.  $\text{PF}_6$  is not solvated by DMSO), we tuned the binding energy to match the experimental results. This was done using

$$\tilde{E}_{\pm} = -2.$$

For completeness, we list all parameters in table [S1](#).

**Table S1: Parameterisation of the KPF<sub>6</sub> in DMSO electrolyte mixture discussed in section V C.**

| Quantity      | Dimension          | Value                 | Source / Method    |
|---------------|--------------------|-----------------------|--------------------|
| $\epsilon_R$  | -                  | 46.7                  | <a href="#">S8</a> |
| $\nu_s$       | mol/m <sup>3</sup> | $1.42 \times 10^{-4}$ | <a href="#">S8</a> |
| $\nu_{\pm}$   | mol/m <sup>3</sup> | $4.1 \times 10^{-4}$  | <a href="#">S9</a> |
| $\lambda_+^m$ | -                  | 4                     | -                  |
| $\lambda_-^m$ | -                  | 0                     | -                  |
| $\tilde{E}_+$ | -                  | -2                    | fitting            |

## S-10 Influence of Dilution and Solvent Size on the Central Extremum of the Differential Capacitance Without Solvation

As we have discussed in the main text, depending upon the parameter landscape spanned by the electrolyte dilution and the relative size of the species molecules, the profile of the differential capacitance has either a camel shape with two local maxima separated by a local minimum, or it has a bell shape with one global maximum. In this section, we discuss the influence of dilution and size asymmetry on the central extremum, which we define as the local minimum in the case of a camel shaped profile and as the global maximum in the case of a bell shaped profile.

We emphasise that according to the convention used throughout this manuscript, experimentally the pzc is can be found by measuring the potential at which the camel-shaped profile of the differential capacitance has it's central minimum in infinitely dilute electrolytes (see section [V D](#)).

The surface plot shown in fig. [S5](#) illustrates the shift of the central extremum in the differential capacitance away from the pzc. This shift depends on the electrolyte dilution  $\varphi$  (y-axis) and the solvent size  $\gamma_s$  (x-axis). Notably, the electrolyte shown here has a large asymmetry in the ion-sizes

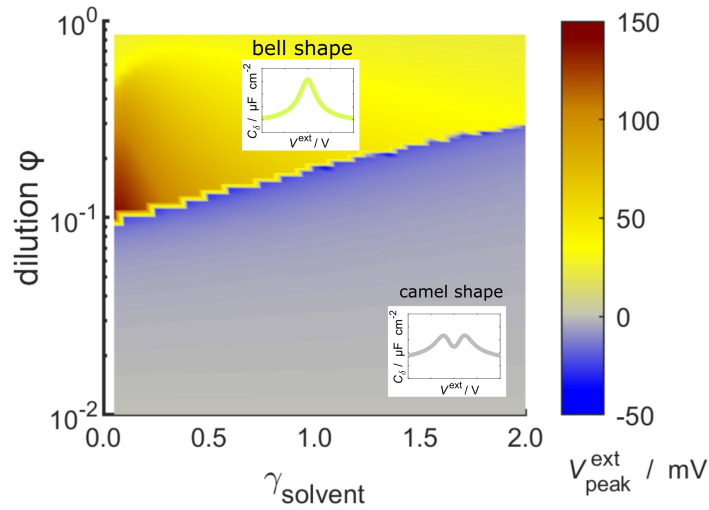

Figure S5: Potential at which the differential capacitance has its central extremum for an asymmetric electrolyte ( $\gamma_+ = 0.9$ ) as a function of dilution  $\varphi$  and solvent size  $\gamma_s$ . The jagged line indicates the switch from a central minimum for low  $\varphi$  (i.e. small salt concentrations) with two neighbouring maxima to a central maximum at higher salt concentrations (indicated on the left axis). For infinitely dilute electrolytes ( $\varphi \rightarrow 0$ ), the central minimum coincides with 0 V.

( $\gamma_+ = 0.9$ ). For comparison, in symmetric electrolytes the central extremum would always lie at  $V^{\text{ext}} = 0$  V.

The surface plot shows the transition from the bell shape to the camel shape as a sharp jagged line stretching from left (at roughly  $\varphi \approx 0.1$ ) to the right (roughly at  $\varphi \approx 0.2$ ). Below that transition line, the region characterised by the colors blue and grey corresponds to the camel shaped case. There, the surface plot illustrates the potential at which  $C_\delta$  has its central minimum. In the limit  $\varphi \rightarrow 0$ , the plot shows the central minimum converges to 0 V, regardless of solvent size. However, if the salt concentration increases, the minimum shifts toward more negative potentials than the pzc (indicated by the blue colouring). This is true for large cations, if the anions were bigger, the shift would be towards positive potentials. In particular, the closer the electrolyte configuration lies to the transition line, the more significant the shift of the central minimum away from 0 V. The most significant discrepancy can be seen just before the step, where the minimum lies more than 20 mV below the pzc. As the critical salt concentration is reached earlier for smaller solvents, either increasing  $\varphi$  or decreasing  $\gamma_s$  increases the misalignment of the central minimum with the

pzc. For electrolyte parameters which correspond to the region above the transition line (marked by yellow and red colors), the differential capacitance has a bell shape. Apparently, the single maximum can shift much further from the pzc than the minimum in the camel-shape case (up to 150 mV). As a general trend, we observe that the global maximum lies closer to the potential of zero charge, the larger the size of the solvent species.

## References

- (S1) Schammer, M. Transport theory for highly correlated electrolytes with non-local species interactions. Ph.D. thesis, Universität Ulm, 2023; <http://dx.doi.org/10.18725/OPARU-50711>.
- (S2) Schammer, M.; Horstmann, B.; Latz, A. Theory of Transport in Highly Concentrated Electrolytes. *Journal of the Electrochemical Society* **2021**, *168*, 026511.
- (S3) Schammer, M.; Latz, A.; Horstmann, B. The Role of Energy Scales for the Structure of Ionic Liquids at Electrified Interfaces: A Theory-Based Approach. *The Journal of Physical Chemistry B* **2022**, *126*, 2761–2776.
- (S4) Kilchert, F.; Lorenz, M.; Schammer, M.; Nürnberg, P.; Schönhoff, M.; Latz, A.; Horstmann, B. A Volume-based Description of Transport in Incompressible Liquid Electrolytes and its Application to Ionic Liquids. *Phys. Chem. Chem. Phys.* **2023**, –.
- (S5) Lorenz, M.; Kilchert, F.; Nürnberg, P.; Schammer, M.; Latz, A.; Horstmann, B.; Schönhoff, M. Local Volume Conservation in Concentrated Electrolytes Is Governing Charge Transport in Electric Fields. *The Journal of Physical Chemistry Letters* **2022**, *13*, 8761–8767.
- (S6) Bazant, M. Z.; Storey, B. D.; Kornyshev, A. A. Double Layer in Ionic Liquids: Overscreening versus Crowding. *Phys. Rev. Lett.* **2011**, *106*, 046102.
- (S7) Kornyshev, A. A. Double-Layer in Ionic Liquids: Paradigm Change? *The Journal of Physical Chemistry B* **2007**, *111*, 5545–5557.

- (S8) Shatla, A.; Landstorfer, M.; Baltruschat, H. On the Differential Capacitance and Potential of Zero Charge of Au(111) in Some Aprotic Solvents. *ChemElectroChem* **2021**, 8, 1817–1835.
- (S9) Pal, T.; Beck, C.; Lessnich, D.; Vogel, M. Effects of Silica Surfaces on the Structure and Dynamics of Room-Temperature Ionic Liquids: A Molecular Dynamics Simulation Study. *The Journal of Physical Chemistry C* **2018**, 122, 624–634.
